# Supplementary material for: Random Field Driven Spatial Complexity at the Mott Transition in VO2
Source: arXiv:1502.05426 source file (2015-02-18)
Supplement: Supplementary file 1 [file supplementary_information.pdf]

# Supplementary Information for: Random Field Driven Spatial Complexity at the Mott Transition in $VO_2$

Shuo Liu, B. Phillabaum, E. W. Carlson, K. A. Dahmen, N. S. Vidhyadhiraja, M. M. Qazilbash, and D. N. Basov

## CRITICAL CLUSTER EXPONENTS

Tables I and II summarize the theoretical values of the critical exponents $\tau$, $d_v$, and $d_h$ (defined in the main text) for the fixed points associated with the disordered Ising model (Eqn. 1 in the paper) [1]. Using cluster analysis techniques, we have derived the experimental value of these critical exponents for a thin film of $VO_2$, in order to determine which fixed point (if any) the experimental system is near.

Our analysis is based on the SNIM data of Ref. [2], taken on a thin film of $VO_2$. The data set is taken from a $4\mu m \times 4\mu m$ area of a 100nm thick film, and the penetration depth of the SNIM is about 20nm [3]. For a slab geometry, exponents will drift from the 3D fixed point toward the associated 2D fixed point, as the correlation length grows beyond the slab thickness. Because the image data is two-dimensional, when comparing the exponents derived from the data with theoretical cluster exponents in any 3D model, we must map the exponents of the 3D model to effective 2D values. For the fractal dimensions $d_v$ and $d_h$, based on the reasonable assumption that at the surface one is observing a 2D cross-section of a 3D cluster, the true fractal dimensions of a 3D model are mapped to the 2D effective values by the geometric factors $d_v \to 2/3 d_v$ and $d_h \to 1/2 d_h$ [1].

For the critical exponent $\tau$ of the cluster size distribution, $D(s) \propto s^{-\tau}$ where $s$ is the mass of a cluster, we find that taking a 2D cross section of a 3D system and using $s \propto R_s^{d_v}$ (where $R_s$ is the radius of gyration) yields [4]

$$\tau_{2Dproj} = \frac{(d\tau - 1)}{(d-1)} - \frac{d}{d_v(d-1)}, \qquad (1)$$

where d is the dimension of the model (in this case $d = 3$), $\tau$ is the true value of the critical exponent for the 3D model itself, and $\tau_{2Dproj}$ is what would be measured in a 2D cross section. By substituting the hyperscaling relation $\tau = (d_v + d)/d_v$ into the equation above, we find that the effective 2D projection of $\tau$ reduces to $\tau_{2Dproj} = (d_v + d)/d_v = \tau$ [4], where $d_v$ is the true (3D) volume fractal dimension. Therefore $\tau_{2Dproj}$ for a 3D model on a 2D projection is the same as $\tau$ for the 3D model itself, and we can directly compare the value of $\tau$ from the data with the theoretical values of 3D models.

In the exponent comparison charts (Fig. 5 in the main text), we have incorporated the above considerations for $\tau$, $d_v$ and $d_h$, using open circles to represent effective 2D projections for 3D fixed points. Thus, for the P-3D and RF-3D fixed points, it is the open circles which should be directly compared with the data-extracted exponents.

## REPRESENTATIVE THRESHOLD AMPLITUDE AND TEMPERATURE

As reported in Ref. [2], in the SNIM images, the metallic regions (light blue, green, and red colors) yield higher near-field scattering amplitude compared with the insulating phase (dark blue color). Thus the threshold amplitude between metallic and insulating is observed to be about $a_{th} = 2.5$, which intersects dark blue and light blue on the color bar of Fig. 2 of Ref. [2].

We also independently determine the threshold amplitude between metallic and insulating regions to be around $a_{th} = 2.5$ using the cluster techniques in this work. Upon varying the threshold $a_{th}$ between our identification of metallic and insulating regions, the cluster pattern changes slightly, and therefore so do the extracted critical exponents. We find, however, that within a broad region around $a_{th} = 2.5$ the critical exponents derived from the data are remarkably robust within error bars, such as shown by the insets of Fig. 3 in the main text. That is, within about 15% of $a_{th} = 2.5$, our cluster exponent results (and therefore our conclusions) are independent of the exact choice of the threshold $a_{th}$. The robustness of the extracted critical exponents to changes in the exact value of the amplitude threshold is consistent with the claim that the system is near a critical point, since universal properties in the neighborhood of a critical point are independent of the microscopic details of the system.

There are six experimental SNIM data images through the Mott transition process, as shown by Fig. 1 in the main text. Among them, $T = 342.6K$, $T = 342.8K$, and $T = 343K$ show spatial complexity with enough clusters for good statistics. These temperatures, compared with others, are closer to the critical end point near the Mott transition. Among them, $T = 342.8K$ appears to be the best intermediate temperature closest to criticality since the corresponding Isingmap in Fig. 1 in the paper shows better spatial complexity of self-similar geometric clusters encompassing different lengthscales in the FOV, implicating most robust scaling behavior. In our cluster analysis, we find that the critical exponents extracted from different intermediate temperatures are unidentifiable from each other within error bars.

Since the data-extracted exponents are universal for different intermediate temperatures throughout the sta-

TABLE I. Theoretical Critical Cluster Exponents of Two Dimensional Ising Models

| Model | Clean Ising Model [5, 6] | Random Bond Disorder [5, 6] | Percolation [7–9] | Random Field Disorder [10–12] |
|---|---|---|---|---|
| Fixed Point | C-2D | C-2D | P-2D | RF-2D |
| $\tau$ | 2.067 | 2.067 | 2.02 | 2.0 |
| $d_v$ | 187/96=1.95 | 187/96=1.95 | 91/48=1.9 | 1.9 |
| $d_h$ | 11/8=1.375 | 11/8=1.375 | 7/4=1.75 | 1.75 |

TABLE II. Theoretical Critical Cluster Exponents of Three Dimensional Ising Models

| Model | Clean Ising Model [13–15] | Random Bond Disorder [15, 16] | Percolation [9, 16–18] | Random Field Disorder [19, 20] |
|---|---|---|---|---|
| Fixed Point | C-3D | RB-3D | P-3D | RF-3D |
| $\tau$ | 2.208 | 2.207 | 2.18 | 2.02±0.03 |
| $d_v$ | - | - | 2.53 | 2.78±0.05 |
| $d_h$ | - | - | 2.5 | 2.11±0.03 |

ble threshold region around $a_{th} = 2.5$, and due to the limited datasets (finite FOV and few data configurations), we use the DLD results under $a_{th} = 2.5$ and $T = 342.8K$ to represent the values of exponents characterizing the spatial complexity. As a double check, from our analysis, for the different intermediate temperatures throughout the threshold region, we find that the main value of $\tau$ is in the range (1.90-1.94) with typically 5% error bar), $d_v$ is in (1.92-1.96) with typically 4% error bar, and $d_h$ is in (1.19-1.23) with typically 3% error bar. They are consistent with the values extracted under the representative condition, and do not introduce any change to our discussions and conclusions through the exponent comparisons.

## ADDITIONAL NOTES FOR $\tau$

Figure 1 shows the power law fit for $\tau$ at T=342.8K with scattering amplitude threshold of $a_{th} = 2.5$. In the figure, $D(s)$ is plotted for all clusters within the FOV, although the fit is done excluding the spanning cluster, because we cannot know *a priori* whether it is in the scaling regime. Power law behavior is evident over 3.5 decades of scaling. This long correlation length is consistent with the system being near a second order critical point. The inset of Fig. 1 shows $\tau$ as a function of threshold amplitude $a_{th}$ for the three intermediate temperatures $342.6K$, $342.8K$ and $343K$, and the common stable minimum region of $\tau$ (with error bars) around $a_{th} = 2.5$ again illustrates that the results of our analysis within error bars are independent of the choice of intermediate temperatures and threshold scattering amplitudes around $a_{th} = 2.5$.

The cluster size distribution exponent $\tau$ obeys the constraint $2 < \tau < 3$ [7]. However, $\tau = 1.532 \pm 0.066$ extracted in Fig. 1 from all clusters in the FOV is significantly smaller than the lower boundary of this constraint.

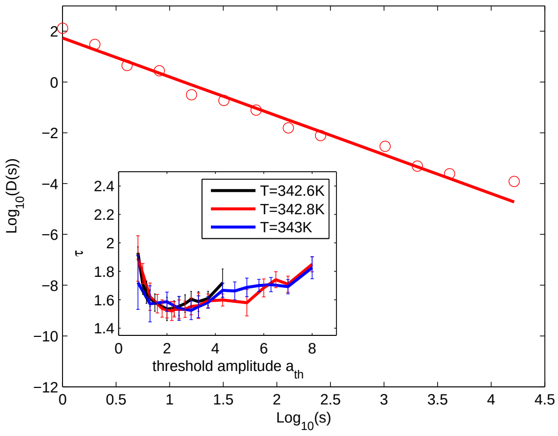


FIG. 1. Power law fit of $D(s) \propto s^{-\tau}$ using all clusters in the Ising map with $a_{th} = 2.5$ at T=342.8K, yielding $\tau = 1.532 \pm 0.066$. The inset shows $\tau$ (with error bars) extracted from all clusters as a function of $a_{th}$ for the three intermediate temperatures.

The reason, as stated in the main text, is that in a finite FOV estimates of $\tau$ are skewed to lower values because of a pronounced scaling bump in the cluster size distribution. Therefore we use the internal clusters in the main text, and $\tau = 1.92 \pm 0.11$ extracted from internal clusters is consistent with the constraint within error bars. The exact estimation of $\tau$ is very difficult in a finite FOV since the cluster size distribution is always affected by the window, which skews the form of power-law scaling behavior. As is evident from the exponent comparison charts (Fig. 4 in the main text), there is a narrow range of theoretical values for $\tau$ displayed by the fixed points. For this reason, it is difficult even in principle to distinguish among the various fixed points based on the value of $\tau$. Nevertheless, the fact that the data-extracted value of $\tau$

from internal clusters is consistent within error bars with the theoretical value of $\tau$ for several Ising fixed points, as shown by Fig. 4 in the paper, indicates that our results are reasonable.

## EXTRACTION OF $d_v$ AND $d_h$

In the relation $s \propto R_s^{d_v}$, the radius of gyration of a cluster, $R_s$, is defined by $2R_s^2 = \sum_{i,j} |\mathbf{r}_i - \mathbf{r}_j|^2/s^2$, where the sum is over all sites in the cluster, and $\mathbf{r}_i$ and $\mathbf{r}_j$ are the positions of site i and site j [9]. In the case of extracting the hull fractal dimension $d_h$, we are only tracking the outer (externally accessible) surfaces of each cluster, thus one surface might contain not only the cluster itself, but also the subclusters inside. Therefore, $R_h$ in the relation $h \propto R_h^{d_h}$ refers to the radius of gyration of *all* the sites enclosed by the hull.

In Fig. 3(b) and 3(c) of the main text, we exclude the first bin from the fit, because it is dominated by non-universal short length scale effects, and also because it includes the $s = 1$ clusters, which from the definition have $R_s = 0$, thus artificially introducing a singularity. Because universality is a long distance feature, excluding this bin will not obscure the form of the power law.

Interestingly, the fractal dimensions do not appear to suffer from the same finite FOV effects as $\tau$. For example, under the representative condition, we find that $d_v$ for all clusters is $1/d_v = 0.514 \pm 0.010$, consistent with $1/d_v = 0.518 \pm 0.020$ for internal clusters. Also, $1/d_h = 0.811 \pm 0.024$ for all clusters is consistent with $1/d_h = 0.829 \pm 0.020$ for internal clusters. In order to avoid the possible finite FOV effect, in the main text we still use the internal clusters for $d_v$ and $d_h$.

## RELATING EXPONENTS TO CLUSTERS AND AVALANCHES

In the paper, we report the critical exponents $\tau$, $d_v$ and $d_h$. These exponents are inferred from the power law scaling behavior entailed by the self-similarity of clusters and avalanches near a critical point, and thus can be directly extracted from the complex patterns revealed by the microscopy imaging experiment. By contrast, exponents such as $\beta$ (the order parameter exponent) and $\nu$ (the correlation length exponent) scale with the relevant variable, and this variable varies from model to model, such as site occupation probability $p - p_c$ in the percolation model, temperature $T - T_c$ in the Ising model, or even disorder strength $R - R_c$ in the random field Ising model. So the values of these exponents are not directly comparable between different models because the relevant variables are different. We don't face such difficulty for $\tau$, $d_v$, and $d_h$, which are extracted explicitly from the spatial complexity itself, and are thus defined in the same way for different models as well as for the image data.

## MICROSCOPIC ORIGIN OF RANDOM FIELD EFFECTS

There are three possible microscopic sources of disorder in these samples: (1) Oxygen defects; (2) Substrate defects; and (3) Grain boundaries. Oxygen defects are unlikely to be a major source of disorder in these samples, since the transition temperature of the film is close to the bulk $T_c$, indicating that the film is quite close to stoichiometric, and we expect defect impurities to be less than 1%. As for substrate defects, the substrate is nearly atomically flat, and so we do not expects significant disorder effects from the substrate.

On the other hand, there are many grain boundaries in the FOV. Since the grains are about $100nm \times 50nm$ in this film [21], and the FOV is $4\mu m \times 4\mu m$, there are about 3000 grains in the FOV. Studies have shown that there is indeed a variation in $T_c$ due to grain size [22]. In addition, our own prior work shows that metallicity nucleates first near the grain boundaries. (See Fig. 6 of Ref. [23] which shows metallic puddles nucleating first on the grain boundaries.)

Now the theoretical consideration becomes whether this type of disorder is of the random field type. On the face of it, since each grain is expected to transition at a slightly different temperature, this is random $T_c$ disorder, which is in the same universality class as random bond disorder. However, physical temperature actually maps to uniform applied field in the model, meaning that in the model, each grain will transition at a different field, and this constitutes therefore random field disorder in the model. One prediction of this line of reasoning is that grain size, since it affects the random field strength in the model, is expected to correlate with the hysteresis width.

## LONG RANGE INTERACTIONS

In passing through the Mott transition, $VO_2$ typically also undergoes a change in lattice structure. (Although see Ref. [24] for a counterexample.) The kind of local lattice rearrangements associated with the clusters observed in the data can introduce strain, and therefore long-range interactions, affecting the universality classes considered. The films under consideration, however, have grains of about $100nm \times 50nm$. The field of view of the dataset in this paper is a $4\mu m \times 4\mu m$ area, which encompasses roughly 40-80 grains along each side of the field of view. The long-range strain effects thus get cut off by the grain size, and the corresponding Ising interactions flow to the short-range case under renormalization group

transformations. Therefore, we compare only to universality classes of short-range Ising models, and our model does not encompass long-range interactions.


[1] B. Phillabaum, E. W. Carlson, and K. A. Dahmen, Nat. Commun. **3**, 915 (2012).
[2] M. M. Qazilbash, M. Brehm, B.-G. Chae, P.-C. Ho, G. O. Andreev, B.-J. Kim, S. J. Yun, A. V. Balatsky, M. B. Maple, F. Keilmann, H.-T. Kim, and D. N. Basov, Science **318**, 1750 (2007).
[3] M. M. Qazilbash, M. Brehm, G. O. Andreev, A. Frenzel, P.-C. Ho, B.-G. Chae, B.-J. Kim, S. J. Yun, H.-T. Kim, A. V. Balatsky, O. G. Shpyrko, M. B. Maple, F. Keilmann, and D. N. Basov, Phys. Rev. B **79**, 075107 (2009).
[4] S. Liu, E. W. Carlson, and K. A. Dahmen, Manuscript in preparation.
[5] J. Cardy, *Scaling and Renormalization in Statistical Physics* (Cambridge University Press, Cambridge, 1996).
[6] W. Janke and A. M. J. Schakel, Phys. Rev. E **71**, 036703 (2005).
[7] D. Stauffer, Phys. Rep. **54**, 1 (1979).
[8] T. Grossman and A. Aharony, J. Phys. A **19**, L745 (1986).
[9] D. Stauffer and A. Aharony, *Introduction to Percolation Theory* (Taylor & Francis, London, 1992).
[10] A. J. Bray and M. A. Moore, J. Phys. C **18**, L927 (1985).
[11] E. T. Seppälä, V. Petäjä, and M. J. Alava, Phys. Rev. E **58**, R5217 (1998).
[12] E. Seppälä, *Ground State Structure, Domain Walls, and External Field Response in Random Magnets*, Ph.D. thesis, Department of Engineering Physics and Mathematics, Helsinki University of Technology (2001).
[13] R. Guida and J. Zinn-Justin, J. Phys. A **31**, 8103 (1998).
[14] A. Coniglio, C. R. Nappi, F. Peruggi, and L. Russo, J. Phys. A **10**, 205 (1977).
[15] V. S. Dotsenko, M. Picco, P. Windey, G. Harris, E. Martinec, and E. Marinari, Nucl. Phys. B **448**, 577 (1995).
[16] P. E. Berche, C. Chatelain, B. Berche, and W. Janke, Eur. Phys. J. B **38**, 463 (2004).
[17] C. D. Lorenz and R. M. Ziff, Phys. Rev. E **57**, 230 (1998).
[18] R. M. Bradley, P. N. Strenski, and J.-M. Debierre, Phys. Rev. B **44**, 76 (1991).
[19] Y. Liu and K. A. Dahmen, Phys. Rev. E **79**, 061124 (2009).
[20] Y. Liu and K. A. Dahmen, Europhys. Lett. **86**, 56003 (2009).
[21] B. G. Chae, H. T. Kim, S. J. Yun, B. J. Kim, Y. W. Lee, D. H. Youn, and K. Y. Kang, Electrochem. Solid-State Lett. **9**, C12 (2006).
[22] E. U. Donev, R. Lopez, L. C. Feldman, and R. F. Haglund, Nano Letters **9**, 702 (2009).
[23] A. Frenzel, M. M. Qazilbash, M. Brehm, B.-G. Chae, B.-J. Kim, H.-T. Kim, A. V. Balatsky, F. Keilmann, and D. N. Basov, Phys. Rev. B **80**, 115115 (2009).
[24] M. K. Liu, M. Wagner, E. Abreu, S. Kittiwatanakul, A. McLeod, Z. Fei, M. Goldflam, S. Dai, M. M. Fogler, J. Lu, S. A. Wolf, R. D. Averitt, and D. N. Basov, Phys. Rev. Lett. **111**, 096602 (2013).
